# Supplementary material for: Manifold Hypothesis: Conditional Certificates and Consistent Intrinsic Dimension Estimation
Source: arXiv:2609.21311 source file (2026-10-16)
Supplement: Supplementary file 1 [file numerical_tables.tex]

\documentclass[10pt]{article}
\usepackage[T1]{fontenc}
\usepackage[margin=.8in]{geometry}
\usepackage{lmodern,amsmath,amssymb,booktabs,float}
\usepackage[hidelinks]{hyperref}
\hypersetup{pdftitle={Numerical supplement to the application-visual revision},pdfauthor={U Jin Choi}}
\renewcommand{\thetable}{S\arabic{table}}
% Keep original source fragments verbatim while fixing their placement here.
\let\originaltable\table
\let\endoriginaltable\endtable
\renewenvironment{table}[1][]{\originaltable[H]}{\endoriginaltable}
\raggedbottom
\begin{document}
\begin{center}
{\Large Numerical supplement to the application-visual revision}\\[6pt]
Manifold Hypothesis: Conditional Certificates and Consistent Intrinsic Dimension Estimation\\[3pt]
U Jin Choi
\end{center}
Tables S1--S4 retain the four exact tables previously consolidated into the main figures. Tables S5--S6 retain the point/ODE and corrected MNIST score tables now displayed as plots. Numerical tabular bodies are unchanged; the MNIST tabular has a new explanatory caption. Placement and numbering differ. These are archived results, with no new experiment or uncertainty estimate. All other numerical tables remain in the manuscript appendices.

\input{tables/rebuiltdirect.tex}
\input{tables/mfmain.tex}
\clearpage
\input{tables/juliadirect.tex}
\input{tables/dimensioncheck.tex}
\clearpage
\input{tables/arxivpoints.tex}
\clearpage
\input{tables/mnist_corrected.tex}
\end{document}
