# Supplementary material for: Manifold Hypothesis: Conditional Certificates and Consistent Intrinsic Dimension Estimation
Source: arXiv:2609.21311 source file (2026-10-16)
Supplement: Supplementary file 2 [file arxivpoints.tex]

\begin{table}[H]\centering\small
\setlength{\tabcolsep}{3pt}
\begin{tabular}{lrrrrrr}\toprule
Model/control & $N$ & $\sigma$ & Returned & Rank 2 & Input error & Output error\\\midrule
Swiss roll & 20,000 & 0.02 & 2000 & 1822 & 0.000497 & 0.003318 \\
Swiss roll & 20,000 & 0.06 & 2000 & 1822 & 0.001437 & 0.003230 \\
Swiss roll & 20,000 & 0.12 & 2000 & 1814 & 0.002960 & 0.003598 \\
Two-torus & 20,000 & 0.02 & 2000 & 1994 & 0.000483 & 0.012288 \\
Two-torus & 20,000 & 0.06 & 2000 & 1997 & 0.001446 & 0.011288 \\
Two-torus & 20,000 & 0.12 & 2000 & 1983 & 0.002835 & 0.010126 \\
Lorenz $\rho=24$ & 1,000 & 0.02 & 1978 & 1384 & 0.000963 & 0.001455 \\
Lorenz $\rho=24$ & 6,000 & 0.02 & 2000 & 1902 & 0.000963 & 0.000995 \\
Lorenz $\rho=24$ & 10,000 & 0.02 & 2000 & 1937 & 0.000963 & 0.000970 \\
Lorenz $\rho=28$ & 1,000 & 0.02 & 1953 & 1187 & 0.000982 & 0.003591 \\
Lorenz $\rho=28$ & 6,000 & 0.02 & 1998 & 1900 & 0.000982 & 0.001155 \\
Lorenz $\rho=28$ & 10,000 & 0.02 & 1999 & 1925 & 0.000982 & 0.001129 \\
Lorenz $\rho=40$ & 1,000 & 0.02 & 1890 & 710 & 0.000956 & 0.010009 \\
Lorenz $\rho=40$ & 6,000 & 0.02 & 1990 & 1821 & 0.000956 & 0.001336 \\
Lorenz $\rho=40$ & 10,000 & 0.02 & 1997 & 1895 & 0.000956 & 0.001216 \\
R\"ossler $c=4$ & 1,000 & 0.02 & 1996 & 90 & 0.000954 & 0.013756 \\
R\"ossler $c=4$ & 6,000 & 0.02 & 2000 & 100 & 0.000954 & 0.013895 \\
R\"ossler $c=4$ & 10,000 & 0.02 & 2000 & 106 & 0.000954 & 0.013760 \\
R\"ossler $c=5.7$ & 1,000 & 0.02 & 1973 & 1001 & 0.000938 & 0.006605 \\
R\"ossler $c=5.7$ & 6,000 & 0.02 & 2000 & 1267 & 0.000938 & 0.003790 \\
R\"ossler $c=5.7$ & 10,000 & 0.02 & 2000 & 1302 & 0.000938 & 0.003431 \\
R\"ossler $c=8.5$ & 1,000 & 0.02 & 1863 & 885 & 0.000954 & 0.003885 \\
R\"ossler $c=8.5$ & 6,000 & 0.02 & 1986 & 1332 & 0.000954 & 0.001441 \\
R\"ossler $c=8.5$ & 10,000 & 0.02 & 1996 & 1409 & 0.000954 & 0.001379 \\
\bottomrule\end{tabular}
\caption{All 24 configurations in the four archived point/ODE figures. Returned and rank-two counts use the full 2,000-query set. Errors are median Euclidean errors in the stated normalized coordinates, conditional on output availability for the projection column. Here $\sigma$ is raw-view coordinate noise standard deviation, applied after the stated normalization. The population-spectral certificate count is zero in every row; geometric certification is unavailable. Input and projection errors retain all adverse comparisons.}
\label{tab:arxivpoints}
\end{table}
