# Supplementary material for: Manifold Hypothesis: Conditional Certificates and Consistent Intrinsic Dimension Estimation
Source: arXiv:2609.21311 source file (2026-10-16)
Supplement: Supplementary file 3 [file dimensioncheck.tex]

\begin{table}[!t]
\centering\small
\caption{Observed-repeat dimension point estimates on $S^2\subset\mathbb R^8$. Each row uses 50 independent simulated inputs; $n$ counts latent groups. Error is the median normalized operator error. Every finite-observation covariance bound was vacuous. These are point-estimator checks, not dimension certificates.}
\label{tab:dimensioncheck}
\begin{tabular}{rrrrr}\toprule
$n$ & $k$ & $r$ & Correct / trials & Median $\|\widehat C-C_x(r)\|/r^2$\\\midrule
256 & 8 & 0.800 & 47/50 & 0.1022\\
1024 & 19 & 0.650 & 50/50 & 0.0723\\
4096 & 43 & 0.528 & 50/50 & 0.0471\\
16384 & 98 & 0.429 & 50/50 & 0.0274\\
\bottomrule\end{tabular}
\end{table}
