# Supplementary material for: Manifold Hypothesis: Conditional Certificates and Consistent Intrinsic Dimension Estimation
Source: arXiv:2609.21311 source file (2026-10-16)
Supplement: Supplementary file 4 [file juliadirect.tex]

\begin{table}[!t]\centering\small
\caption{New Julia direct-coordinate runs, distinct from Table~\ref{tab:mfmain}. Each row has 10 independent inputs. The three support targets are paired checks on those same inputs. RMS errors average the per-trial Euclidean RMS over all 16,384 latent groups in $\mathbb R^{16}$.}
\label{tab:juliadirect}
\begin{tabular}{rrrrrrr}\toprule
 & \multicolumn{3}{c}{Support emissions at tolerance} & Reported & \multicolumn{2}{c}{Mean RMS error}\\
$k$ & $0.6$ & $0.9$ & $1.3$ & bound range & Means & Decoded\\\midrule
16 & 0/10 & 0/10 & 10/10 & 0.9921--1.0090 & 0.06002 & 0.01506\\
64 & 0/10 & 0/10 & 10/10 & 0.9369--0.9468 & 0.03001 & 0.00754\\
256 & 0/10 & 0/10 & 10/10 & 0.9102--0.9146 & 0.01500 & 0.00376\\
\bottomrule\end{tabular}\end{table}
