# Supplementary material for: Manifold Hypothesis: Conditional Certificates and Consistent Intrinsic Dimension Estimation
Source: arXiv:2609.21311 source file (2026-10-16)
Supplement: Supplementary file 5 [file mfmain.tex]

\begin{table}[!t]
\centering\small
\caption{Executed rational certificates: emissions out of 30. The fixed tube radius is $0.12$; support tolerances are $0.3$ (Moons) and $1.3$ (Julia).}
\label{tab:mfmain}
\begin{tabular}{lrr}\toprule
Condition & Support & Mass\\\midrule
Moons, $\sigma=0.02$ & 30/30 & 30/30\\
Moons, $\sigma=0.06$ & 30/30 & 30/30\\
Moons, $\sigma=0.12$ & 30/30 & 30/30\\
Moons, $\sigma=0.24$ & 0/30 & 0/30\\
Julia, $k=16$ & 30/30 & 0/30\\
Julia, $k=64$ & 30/30 & 30/30\\
Julia, $k=256$ & 30/30 & 30/30\\
\bottomrule\end{tabular}
\end{table}
