# Supplementary material for: Manifold Hypothesis: Conditional Certificates and Consistent Intrinsic Dimension Estimation
Source: arXiv:2609.21311 source file (2026-10-16)
Supplement: Supplementary file 6 [file mnist_corrected.tex]

\begin{table}[H]\centering
\begin{center}\small
\begin{tabular}{@{}cc l rrrr@{}}\toprule
$\sigma$ & $k$ & Method & MSE & PSNR & SSIM & Fail/120\\\midrule
$0.10$ & 4 & Repeat mean & 0.002499 & 26.027 & 0.7810 & 0 \\
$0.10$ & 4 & PCA64 only & 0.009322 & 20.593 & 0.7349 & 0 \\
$0.10$ & 4 & Local PCA64 & 0.016347 & 18.440 & 0.6602 & 0 \\
$0.10$ & 4 & Yao--Xia objective & 0.014631 & 18.916 & 0.6846 & 0 \\
$0.10$ & 4 & Native LPCA784 & 0.007011 & 22.633 & 0.7849 & 0 \\
$0.20$ & 4 & Repeat mean & 0.009997 & 20.007 & 0.6938 & 0 \\
$0.20$ & 4 & PCA64 only & 0.009996 & 20.251 & 0.7139 & 0 \\
$0.20$ & 4 & Local PCA64 & 0.016584 & 18.349 & 0.6532 & 0 \\
$0.20$ & 4 & Yao--Xia objective & 0.014937 & 18.771 & 0.6733 & 0 \\
$0.20$ & 4 & Native LPCA784 & 0.007457 & 21.797 & 0.7475 & 0 \\
$0.40$ & 4 & Repeat mean & 0.039989 & 13.986 & 0.5811 & 0 \\
$0.40$ & 4 & PCA64 only & 0.012697 & 19.125 & 0.6620 & 0 \\
$0.40$ & 4 & Local PCA64 & 0.017824 & 17.958 & 0.6281 & 0 \\
$0.40$ & 4 & Yao--Xia objective & 0.017000 & 18.157 & 0.6362 & 0 \\
$0.40$ & 4 & Native LPCA784 & 0.019676 & 17.394 & 0.6070 & 1 \\
$0.20$ & 1 & Repeat mean & 0.039723 & 14.014 & 0.5817 & 0 \\
$0.20$ & 1 & PCA64 only & 0.012715 & 19.120 & 0.6615 & 0 \\
$0.20$ & 1 & Local PCA64 & 0.016589 & 18.114 & 0.6556 & 17 \\
$0.20$ & 1 & Yao--Xia objective & 0.016597 & 18.193 & 0.6397 & 0 \\
$0.20$ & 1 & Native LPCA784 & 0.019686 & 17.395 & 0.6065 & 0 \\
\bottomrule\end{tabular}
\end{center}
\caption{Corrected synthetic-noise MNIST scores. The original numerical tabular is retained verbatim. All 120 image--seed cases use unclipped scores with explicitly flagged fallback for undefined outputs. Native LPCA784 is a separate preprocessing/rank diagnostic.}
\label{tab:mnistcorrectedexact}
\end{table}
