# Supplementary material for: Manifold Hypothesis: Conditional Certificates and Consistent Intrinsic Dimension Estimation
Source: arXiv:2609.21311 source file (2026-10-16)
Supplement: Supplementary file 7 [file rebuiltdirect.tex]

\begin{table}[H]\centering\small
\setlength{\tabcolsep}{4pt}
\caption{Paired algorithm revision on the same 60 archived observations. Bounds and RMS errors are means across ten trials. Emissions use the unchanged primary tolerance $1.2$. The $k=4$ witness reconstructions are diagnostics after abstention.}\label{tab:rebuiltdirect}
\begin{tabular}{@{}lrrrrrrr@{}}\toprule
Support & $k$ & Old bound & New bound & Old emit & New emit & Span RMS & Witness RMS\\\midrule
Torus & 4 & 1.7760 & 1.7423 & 0/10 & 0/10 & 0.1039 & 0.0852\\
Torus & 64 & 1.1704 & 1.0711 & 10/10 & 10/10 & 0.0260 & 0.0212\\
Torus & 256 & 1.0772 & 0.9804 & 10/10 & 10/10 & 0.0130 & 0.0106\\
Torus + branch & 4 & 1.9385 & 1.7456 & 0/10 & 0/10 & 0.1040 & 0.0882\\
Torus + branch & 64 & 1.4351 & 1.0774 & 0/10 & 10/10 & 0.0260 & 0.0314\\
Torus + branch & 256 & 1.3569 & 0.9861 & 0/10 & 10/10 & 0.0130 & 0.0266\\
\bottomrule\end{tabular}\end{table}
